# Supplementary material for: Minimalist Vision with Freeform Pixels
Source: arXiv:2501.00142 source file (2024-12-30)
Supplement: Supplementary file 1 [file supp.tex]

\documentclass[runningheads]{llncs}

% ---------------------------------------------------------------
% Include basic ECCV package
 
% TODO REVIEW: Insert your submission number below by replacing '*****'
% TODO FINAL: Comment out the following line for the camera-ready version
% \usepackage[review,year=2024,ID=8113]{eccv}
% TODO FINAL: Un-comment the following line for the camera-ready version
\usepackage{eccv}

% OPTIONAL: Un-comment the following line for a version which is easier to read
% on small portrait-orientation screens (e.g., mobile phones, or beside other windows)
%\usepackage[mobile]{eccv}

% ---------------------------------------------------------------
% Other packages

% Commonly used abbreviations (\eg, \ie, \etc, \cf, \etal, etc.)
\usepackage{eccvabbrv}

% Include other packages here, before hyperref.
\usepackage{graphicx}
\usepackage{booktabs}
\usepackage{siunitx}
\usepackage{amsmath}
\usepackage{comment}
\usepackage{afterpage}
\usepackage{import}
\usepackage{wrapfig}
\usepackage{multirow}

% The "axessiblity" package can be found at: https://ctan.org/pkg/axessibility?lang=en
\usepackage[accsupp]{axessibility}  % Improves PDF readability for those with disabilities.

% ---------------------------------------------------------------
% Hyperref package

% It is strongly recommended to use hyperref, especially for the review version.
% Please disable hyperref *only* if you encounter grave issues.
% hyperref with option pagebackref eases the reviewers' job, but should be disabled for the final version.
%
% If you comment hyperref and then uncomment it, you should delete
% main.aux before re-running LaTeX.
% (Or just hit 'q' on the first LaTeX run, let it finish, and you
%  should be clear).

% TODO FINAL: Comment out the following line for the camera-ready version
% \usepackage[pagebackref,breaklinks,colorlinks]{hyperref}
% TODO FINAL: Un-comment the following line for the camera-ready version
\usepackage{hyperref}

% Support for ORCID icon
\usepackage{orcidlink}

\input{macros}

\setlength{\tabcolsep}{6pt}

\begin{document}

% ---------------------------------------------------------------
% TODO REVIEW: Replace with your title
\title{Minimalist Vision with Freeform Pixels: Supplemental Material}

% TODO REVIEW: If the paper title is too long for the running head, you can set
% an abbreviated paper title here. If not, comment out.
% \titlerunning{Minimalist Vision with Freeform Pixels}

% TODO FINAL: Replace with your author list. 
% Include the authors' OCRID for the camera-ready version, if at all possible.
\author{
Jeremy Klotz%\orcidlink{0009-0005-9408-3541}
\and Shree K. Nayar%\orcidlink{0000-0002-6452-6998}
}

% TODO FINAL: Replace with an abbreviated list of authors.
\authorrunning{J.~Klotz \and S.K.~Nayar}
% First names are abbreviated in the running head.
% If there are more than two authors, 'et al.' is used.

% TODO FINAL: Replace with your institution list.
\institute{
Computer Science Department, Columbia University, New York NY, USA
\email{\{jklotz,nayar\}@cs.columbia.edu}
}

\maketitle

\input{supplemental/sec01_sensor_model}

\input{supplemental/sec02_hardware_description}

\input{supplemental/sec03_experiments}

% ---- Bibliography ----
%
% BibTeX users should specify bibliography style 'splncs04'.
% References will then be sorted and formatted in the correct style.
%
\bibliographystyle{splncs04}
\bibliography{Mincam}
\end{document}
